# Supplementary material for: Minimizing Multimodular Functions and Allocating Capacity in Bike-Sharing Systems
Source: arXiv:1611.09304 source file (2022-03-14)
Supplement: Supplementary file 1 [file appendix_scaling_lemma_old.tex]

\subsubsection{Proof of Lemma \ref{lem:phase_bound}}

By Theorem \ref{thm: koptimal}, the number of dock-moves required in each iteration is the minimum number of dock-moves with which an optimal allocation (for that phase) could be obtained. We argue that the dock-move distance between optimal allocations in two subsequent phases cannot be too large. Notice first that if a phase requires $L>4n$ dock-moves, then the pigeonhole principle implies that there must exist a sequence of dock-moves of length $L$ that leads to the same allocation and involves the exact same dock-move twice. For example, if the moves $e_{ij}$, $e_{kj}$ and $e_{i\ell}$ occur, then the moves $e_{ij},e_{ij}$, and $e_{k\ell}$ yield the same changes, but involve $e_{ij}$ twice. The same argument holds for the other kinds of moves. By Theorem~\ref{thm: koptimal}, carrying out all of the $L$ moves except for the two $e_{ij}$ cannot yield the optimal objective for this phase. Thus, beginning the phase with all but those two moves, we find a suboptimal allocation such that doing the $e_{ij}$ does yield an optimal allocation; this implies in particular that the $e_{ij}$ yield improvement at that point. Now, notice that beginning the phase (before moving to a bike-optimal allocation) with the two $e_{ij}$ moves cannot yield improvement as it gives an allocation that would have been feasible in the last phase.
 
 We now want to bound the improvement of the two moves at the end in terms of the improvement at the beginning. While multimodularity implies diminishing returns in each iteration of the gradient-descent algorithm, this relies on the allocations being bike-optimal. Though the allocation at the beginning of the phase may not be bike-optimal (for the permitted number of bikes to be moved in each iteration of {\em this} phase), it cannot be more than $n$ bike-moves away from being bike-optimal. This allows us to count each dock-move occurring in that phase as either one of the at most $4n$ moves with no duplicates or as one of the at most $n$ moves before improvements of subsequent moves are at most what they were prior to moving to bike-optimal. Combining the two bounds, we derive a contradiction from $L>5n$ and thus prove the lemma.\qed
 
 \subsubsection{Extension to operational constraints}
 
 While the same ideas as in Lemma \ref{lem:phase_bound} still work in the presence of constraints on the number of docks moved, we need to be careful to ensure that in each phase we remain within $S_z(\vec{d},\vec{b})$. We adapt the scaling algorithm in the following way to ensure this (cf. Algorithm \ref{alg:scaling_ops}): rather than starting each new phase at the optimal solution found in the last phase, we move that solution closer to the current solution and initiate the discrete-gradient descent steps from that new solution. Suppose in the last iteration we found a solution at distance $z$ from the current allocation that is optimal when only allowing multiples of $2^k$ to be moved; in order to find the optimal solution when allowing multiples of $2^{k-1}$, we %For this to yield a polynomial-time algorithm we require that starting with a solution that is at distance $z$ from the current allocation and optimal for the phase in which $2^k$ docks/bikes are moved in each step, 
 require the existence of a number $M$ such that (i) $M$ is polynomial in $n$, (ii) the new starting point of the phase is in $S_{z-2^{k-1}M}(\vec{d},\vec{b})$, and (iii) there exists an optimal solution within $S_z(\vec{d},\vec{b})$, for steps involving $2^{k-1}$ docks/bikes each, that is at most $M$ such steps away from the new starting point. By Theorem \ref{thm: koptimal}, running $M$ gradient descent steps then finds an optimal solution within $S_{z}(\vec{d},\vec{b})$ in the new phase.
 
 \begin{lemma}
Let $(\vec{d}^k,\vec{b}^k)$ be the optimal solution found in the phase in which we move $2^k$ docks/bikes in each iteration and let $(\vec{d}^{k-1},\vec{b}^{k-1})$ be the optimal solution for the subsequent phase that is closest (in dock-move distance) to $(\vec{d}^k,\vec{b}^k)$. Let $\alpha$ denote that dock-move distance (counting the number of moves of $2^{k-1}$ docks/bikes each). We define $(\vec{d}',\vec{b}')$ by setting:
\begin{itemize}
    \item if $d_i^k+b_i^k \geq \bar{d_i}+\bar{b_i}$, then $d_i'+b_i'=\max\{d_i^k+b_i^k-\alpha2^{k-1}, \bar{d_i}+\bar{b_i}\}$
    \item if $d_i^k+b_i^k < \bar{d_i}+\bar{b_i}$, then $d_i'+b_i'=\min\{d_i^k+b_i^k+\alpha2^{k-1}, \bar{d_i}+\bar{b_i}\}$.
\end{itemize}
Then, as long as $\alpha$ is polynomial in $n$, $M=\frac{\sum_i|d_i'+b_i'-d_i^k+b_i^k|}{2^k}$ fulfills properties (i)-(iii) above.
 \end{lemma}

\emph{Proof.} Property (i) holds with $M\leq \alpha n$; (ii) holds because each of the $M$ docks moved from $(\vec{d}^k,\vec{b}^k)$ to $(\vec{d}',\vec{b}')$ decreases the move-distance from the current allocation. We need to argue that property (iii) holds as well by showing that the dock-move distance from $(\vec{d}',\vec{b}')$ to $(\vec{d}^{k-1},\vec{b}^{k-1})$ is at most $M$.

Notice first that there is no station $i$ such that either 
\begin{itemize}
    \item $d'_i+b'_i<\bar{d}_i+\bar{b}_i$ and $d^{k-1}_i+b^{k-1}_i>\bar{d}_i+\bar{b}_i$ or
    \item $d'_i+b'_i>\bar{d}_i+\bar{b}_i$ and $d^{k-1}_i+b^{k-1}_i<\bar{d}_i+\bar{b}_i$.
\end{itemize}
In fact, if there was such a location $i$, then $d^{k-1}_i+b^{k-1}_i$ would have to be greater than $\alpha$ moves (of step-size $2^{k-1}$) away from $d^{k}_i+b^{k}_i$, contradicting the distance being $\alpha$. We deduce that
$$
\sum_i |d_i+b_i-d_i'-b_i'| + |d_i'+b_i' - d_i^{k-1}-b_i^{k-1}|
= \sum_i |d_i+b_i- d_i^{k-1}-b_i^{k-1}| \leq z.
$$
Since $\sum_i |d_i+b_i-d_i'-b_i'| = z-M$, it follows that $\sum_i |d_i'+b_i' - d_i^{k-1}-b_i^{k-1}|\leq M$ which concludes the proof of the Lemma. \qed
%the triangle inequality in distance from the current allocation to $(\vec{d}',\vec{b}')$ and from $(\vec{d}',\vec{b}')$ to $(\vec{d}^{k-1},\vec{b}^{k-1})$ holds with equality; thus, given that $(\vec{d}^{k-1},\vec{b}^{k-1})$ is at most $z$ steps away from the current allocation and $(\vec{d}',\vec{b}')$ being $z-M$ steps away from the current allocation, we deduce that $(\vec{d}',\vec{b}')$ and $(\vec{d}^{k-1},\vec{b}^{k-1})$ are at most $M$ steps away from each other. 

By Lemma \ref{lem:phase_bound}, $\alpha\in O(n)$ when there are no \emph{operational} constraints. We next show that, a looser bound of $\alpha\in O(n^3)$ can be obtained when we do have these constraints.

 \begin{lemma}
With $(\vec{d}^k,\vec{b}^k)$ and $(\vec{d}^{k-1},\vec{b}^{k-1})$ defined as in the last lemma, the dock-move distance between the two, where each move involves $2^{k-1}$ docks/bikes, is bounded by $O(n^3)$.
 \end{lemma}
\emph{Proof. } %We choose the bound intentionally loose to give a simpler argument. The argument in Lemma \ref{lem:phase_bound} breaks down when the identified move leads to a solution violating the dock-move constraints. 
Similar to Lemma \ref{lem:phase_bound} we again use a pigeonhole argument, however, this time we bucket each individual dock-move, i.e., for each pair/triple $(i,j)$/$(i,j,h)$ we consider all possible moves. A loose bound on the number of moves before duplicates arise is $4n^3$ (without the bucketing arguments we used in Lemma \ref{lem:phase_bound}). Recall that the dock-move distance to the current allocation is assumed to be the same for $(\vec{d}^k,\vec{b}^k)$ and $(\vec{d}^{k-1},\vec{b}^{k-1})$. Suppose $\beta$ among the moves in the path from $(\vec{d}^k,\vec{b}^k)$ to $(\vec{d}^{k-1},\vec{b}^{k-1})$ appear once and do not increase, or even decrease the dock-move distance to the current allocation. Then there can be at most $\beta$ moves that increase the dock-move distance to the current. Further, there can be no repeated moves that decrease the dock-move distance, as we can combine two iterations of such a move and two iterations of a move that decreases the dock-move distance, to find a feasible solution in the previous phase. By the same argument as in Lemma \ref{lem:phase_bound}, that solution would contradict the optimality of $(\vec{d}^k,\vec{b}^k)$ in the previous phase. Thus, we know that $\beta\leq 4n^3$ as otherwise duplicates would occur; but then, there can be no more than $8n^3$ moves in the path from $(\vec{d}^k,\vec{b}^k)$ to $(\vec{d}^{k-1},\vec{b}^{k-1})$. \qed

%$(\vec{d}^k,\vec{b}^k)$ to $(\vec{d}^{k-1},\vec{b}^{k-1})$
%any move decreasing the dock-move If we had $Z\leq 4n^3$, we know that the total number of moves is at most $$ we know that
%If no such move exists (i.e., no two moves that do not increase the dock-move distance when performed at 
In this section we assumed so far that in each phase we search for the optimal solution at the same distance from the current allocation as in the last phase; in particular, we assumed that the distance from the current allocation is the same for the optimal solution in consecutive phases. In practice, we may have optimal solutions $O(n)$ moves further from the current allocation (by a similar argument as in Lemma \ref{lem:phase_bound}, e.g., if the bounds at each station do not allow us to add an additional $2^k$ docks, but do allow us to add an additional $2^{k-1}$ docks). In that case, we may first find an optimal solution with moves of size $2^{k-1}$ for the distance in the last phase, and then carry out an additional number of moves, linear in $n$, to find the solution for the actual distance constraint. Combining these ideas we obtain a polynomial-time algorithm for the optimization problem.

\begin{theorem}
Algorithm \ref{alg:scaling_ops} runs in time polynomial in $n$ and $\log(B+D)$.
\end{theorem}
%But that means that first finding the optimal solution within $S_z$ (where $z$ is the distance in the last phase), followed by another $n$ gradient-descent steps, %is at the same distance from the current allocation as the solution found in the previous phase and the

%The above arguments yield a polynomial-time algorithm to find an optimal solution in $S_z(\vec{d},\vec{b})$.
%The lacking piece to a polynomial-time algorithm is that the solution $(\vec{d}^{k-1},\vec{b}^{k-1})$ is at the same distance $z$ from the current allocation as the one in the previous phase; however, in the new phase, an optimal solution could be up to $n2^{k-1}$ further away; so we may have to run the gradient-descent algorithm for up to $M+n$ iterations. But that's still fine!



% is below d_c and d_k is above or vice-versa; in fact, if there was, then d_{k-1} would have been more than 5n away from d_k initially. I'd like to claim that this guarantees that d_{k-1} is at most M steps away from d_k' - I have a picture, but I can't quite formalize it. 
