# Supplementary material for: Minimizing Multimodular Functions and Allocating Capacity in Bike-Sharing Systems
Source: arXiv:1611.09304 source file (2022-03-14)
Supplement: Supplementary file 2 [file old_appendix_proof_lemma_3.tex]

For the proofs of lemmas \ref{lemma: neighborhoods}--\ref{lemma:const_neighborhood} it is particularly useful to adopt the \emph{diminishing return} interpretation of the multimodular inequalities in Figure \ref{fig:inequalities}. %Two arrows of the same color  compare the improvement of one increment of the same resource (e.g., one additional empty dock, one extra bike) starting from two different locations. 
For example, Inequality (6) implies that when starting from $(1,5)$ the improvement in the UDF at a station is greater when an empty dock is added than when starting from $(1,6)$. Similarly, Inequality (3) means that among two stations with equal capacity, one with more bikes benefits more from an empty dock. The proofs of the two lemmas are building on these properties by comparing the improvements of the same change for different allocations.




\subsubsection{Proof of Lemma \ref{lemma: neighborhoods}}
We first argue that we may assume without loss of generality that there is no solution $(\vec{d}^{\star\star},\vec{b}^{\star\star})$ in the neighborhood of $(\vec{d}^\star,\vec{b}^\star)$ that has better objective than $(\vec{d},\vec{b})$ does and is closer to $(\vec{d},\vec{b})$ in dock-move distance than $(\vec{d}^\star,\vec{b}^\star)$ is. Indeed, if such a solution existed, then it would have to be the case that $(\vec{d}^{\star\star},\vec{b}^{\star\star})$ is component-wise in between $(\vec{d},\vec{b})$ and $(\vec{d}^\star,\vec{b}^\star)$, i.e., for every $i$ we have either $d_i+b_i \leq d_i^{\star\star}+b_i^{\star\star}\leq d_i^{\star}+b_i^{\star}$ or $d_i+b_i \geq d_i^{\star\star}+b_i^{\star\star}\geq d_i^{\star}+b_i^{\star}$. But then, a dock-move from $(\vec{d},\vec{b})$ towards $(\vec{d}^{\star\star},\vec{b}^{\star\star})$ also reduces the dock-move distance to $(\vec{d}^{\star},\vec{b}^{\star})$. If such $(\vec{d}^{\star\star},\vec{b}^{\star\star})$ existed we may relabel it as $(\vec{d}^{\star},\vec{b}^{\star})$, and argue the result for $(\vec{d},\vec{b})$ and this new $(\vec{d}^{\star},\vec{b}^{\star})$ instead (implying the result for the original $(\vec{d}^{\star},\vec{b}^{\star})$).
%induct on $(\vec{d}^{\star\star},\vec{b}^{\star\star})$.


%$(\vec{d}^\star,\vec{b}^\star)$ minimizes the dock-move distance to $(\vec{d},\vec{b})$ among solutions with lower function value than  $(\vec{d},\vec{b})$, i.e., among all $(\vec{d}^\star,\vec{b}^\star)$ such that $\sum_i d_i+b_i=\sum_i d_i^\star+b_i^\star$, $\sum_i b_i = \sum_i b_i^\star$, and $c(\vec{d}^\star,\vec{b}^\star)<c(\vec{d},\vec{b})$, $(\vec{d}^{\star},\vec{b}^{\star})$ has minimum dock-move distance to $(\vec{d},\vec{b})$.


Now, the proof of the lemma follows a case-by-case analysis; since $(\vec{d},\vec{b})$ is assumed to be bike-optimal, for $(\vec{d}^\star,\vec{b}^\star)$ to have a lower objective value it must have a different allocation of docks than $(\vec{d},\vec{b})$ does, i.e., there must be stations $j$ and $k$ such that $j$ has fewer docks in $(\vec{d},\vec{b})$ and $k$ has too many ($d_j+b_j<d_j^\star+b_j^\star$ and $d_k+b_k>d_k^\star+b_k^\star$). We show that in each of the following cases either there exists a dock-move to $j$, or one from $k$, that improves the objective: % or there exists a solution $(\vec{d}^{\star\star},\vec{b}^{\star\star})$ with objective value lower than $(\vec{d},\vec{b})$, $\sum_i d_i+b_i=\sum_i d_i^{\star\star}+b_i^{\star\star}$, and $\sum_i b_i = \sum_i b_i^{\star\star}$, such that $(\vec{d}^{\star\star},\vec{b}^{\star\star})$ is one dock-move closer to $(\vec{d},\vec{b})$ than is $(\vec{d}^\star,\vec{b}^\star)$. \dfedit{As argued above, we may assume without loss of generality that no such $(\vec{d}^{\star\star},\vec{b}^{\star\star})$ exists}; \dfedit{thus, we infer that starting from $(\vec{d},\vec{b})$} there must be a dock-move to $j$ or one from $k$ that yields a lower objective.
%We consider the following cases:

%\dfedit{PARALLELISM BETWEEN 3 AND 4?}

\OneAndAHalfSpacedXI
\begin{enumerate}
\item $j$ has too few empty docks in $(\vec{d},\vec{b})$ and $k$ has too many ($d_j<d_j^\star$ and $d_k>d_k^\star$);
%j needs a bike with a dock
\item $j$ has too few full docks in $(\vec{d},\vec{b})$ and $k$ has too many ($b_j<b_j^\star$ and $b_k>b_k^\star$);
\item $j$ has too few empty, enough full docks, $k$ has too many full docks ($d_j<d_j^\star$, $b_j\geq b_j^\star$, and $b_k>b_k^\star$)
\begin{enumerate}
\item and there exists $\ell$ with $d_\ell+b_\ell< d_\ell^\star+b_\ell^\star$, $b_\ell<b_\ell^\star$;
\item and there exists $\ell$ with $d_\ell+b_\ell\geq d_\ell^\star+b_\ell^\star$, $b_\ell<b_\ell^\star$;
\item for all $\ell\not\in\{j,k\}$, we have $b_{\ell}\geq b_{\ell}^\star$, so $\sum_i b_i>\sum_i b_i^\star$;
\end{enumerate}
\item $j$ has enough empty, too few full docks, $k$ has too few full docks $d_j\geq d_j^\star$, $b_j<b_j^\star$, and $b_k\leq b_k^\star$% $b_k\leq b_k^\star$, and $d_k> d_k^\star$,
\begin{enumerate}
\item and there exists $\ell$ with $d_\ell+b_\ell>d_\ell^\star+b_\ell^\star$ and $b_\ell>b_\ell^\star$;
\item and there exists $\ell$ with $d_\ell+b_\ell\leq d_\ell^\star+b_\ell^\star$ and $b_\ell>b_\ell^\star$;
\item for all $\ell\not\in\{j,k\}$, we have $b_\ell\leq b_\ell^\star$, so $\sum_i b_i<\sum_i b_i^\star$.
\end{enumerate}
\end{enumerate}
\DoubleSpacedXI

\noindent We show that in Case 1.) $c(o_{kj}(\vec{d},\vec{b}))<c(\vec{d},\vec{b})$, i.e., moving an empty dock from $k$ to $j$ yields improvement. The proof for Case 2.) is symmetric using $e_{kj}$ instead. 
Further, the results in~3.a) and~4.a) both reduce to Case~2.). Specifically, $\ell$ in~3.a) fulfills the conditions of $j$ in~2.), and $k$ in~3.a) fulfills $b_k>b_k^\star$, so in~3.a)~$e_{k\ell}$ yields improvement. Similarly, $\ell$ in 4.a) fulfills the conditions of $k$ in~2.), and $j$ in 4.a) fulfills $b_j<b_j^\star$, so in 4.a) $e_{\ell j}$ yields improvement. % there exists a move from~$k$ to~$\ell$ that yields improvement. Similarly, from the result in case~2.), we know that in case~4.a) there must exist a move from $\ell$ to $j$ that yields improvement}. 
The proofs for cases 3.b) and 4.b) are also symmetric with $O_{kj\ell}$ yielding improvement in the former and $E_{kj\ell}$ yielding improvement in the latter; thus, we only present the proof for 3.b). Cases 3.c) and 4.c) violate the constraint $\sum_i b_i = B= \sum_i b_i^\star$ and can thus be excluded.


For Case 1.), we define $(\vec{d}^{\star\star},\vec{b}^{\star\star})=o_{jk}(\vec{d}^{\star},\vec{b}^{\star})$, so 

\vspace{-.35in}
\[
c(\vec{d^{\star\star}},\vec{b}^{\star\star})-c(\vec{d}^{\star},\vec{b}^{\star})
=c_j(d_j^{\star}-1,b_j^{\star})-c_j(d_j^{\star},b_j^{\star}) + c_k(d_k^{\star}+1,b_k^{\star})-c_k(d_k^{\star},b_k^{\star}).
\]

%\vspace{-.1in}

\noindent We argued at the beginning of this proof that we may assume without loss of generality that there exists no solution in the neighborhood of $(\vec{d}^\star,\vec{b}^\star)$ that has better objective than $(\vec{d},\vec{b})$ does and is closer to $(\vec{d},\vec{b})$ in dock-move distance than $(\vec{d}^\star,\vec{b}^\star)$ is. Since $(\vec{d}^{\star\star},\vec{b}^{\star\star})=o_{jk}(\vec{d}^\star,\vec{b}^\star)$, we know that (i)~$(\vec{d}^\star,\vec{b}^\star)$ is closer to $(\vec{d},\vec{b})$ in dock-move distance than $(\vec{d}^\star,\vec{b}^\star)$, and (ii)~$(\vec{d}^{\star\star},\vec{b}^{\star\star})\in N(\vec{d}^{\star},\vec{b}^{\star})$. %and $\sum_i |d_i+b_i-d_i^\star-b_i^\star|>\sum_i |d_i+b_i-d_i^{\star\star}-b_i^{\star\star}|$ 
Then we must have
%this implies that 
$c(\vec{d}^\star,\vec{b}^\star)< c(\vec{d},\vec{b})\leq c(\vec{d}^{\star\star},\vec{b}^{\star\star})$. Thus, by setting $(\vec{d'},\vec{b'})=o_{kj}(\vec{d},\vec{b})$, we obtain the equalities and the final inequality in

\OneAndAHalfSpacedXI
\begin{eqnarray*}
c(\vec{d},\vec{b})-c(\vec{d'},\vec{b'}) =\Big(c_j(d_j,b_j)-c_j(d_j+1,b_j)\Big) + \Big(c_k(d_k,b_k) - c_k (d_k-1,b_k)\Big) \\
\geq \Big(c_j(d_j^{\star}-1,b_j^{\star})-c_j(d_j^{\star},b_j^{\star})\Big) + \Big(c_k(d_k^{\star}+1,b_k^{\star})-c_k(d_k^{\star},b_k^{\star})\Big)
= c(\vec{d}^{\star\star},\vec{b}^{\star\star})-c(\vec{d}^{\star},\vec{b}^{\star})>0.
\end{eqnarray*}

\DoubleSpacedXI
\vspace{-.15in}
\noindent We prove the inequality between the lines by comparing the differences involved, starting with% it holds for each difference, starting with

\vspace{-.25in}
\[
c_j(d_j,b_j)-c_j(d_j+1,b_j)\geq c_j(d_j^{\star}-1,b_j^{\star})-c_j(d_j^{\star},b_j^{\star}).
\]
We refer the reader to Figure \ref{fig:lemma_3} for a graphical presentation of the sequence of inequalities from Definition \ref{def: multimod} we apply (thicker arrows correspond to greater improvement of an added empty dock).
\begin{figure}[ht]
    \centering
    \includegraphics[width=.5\textwidth]{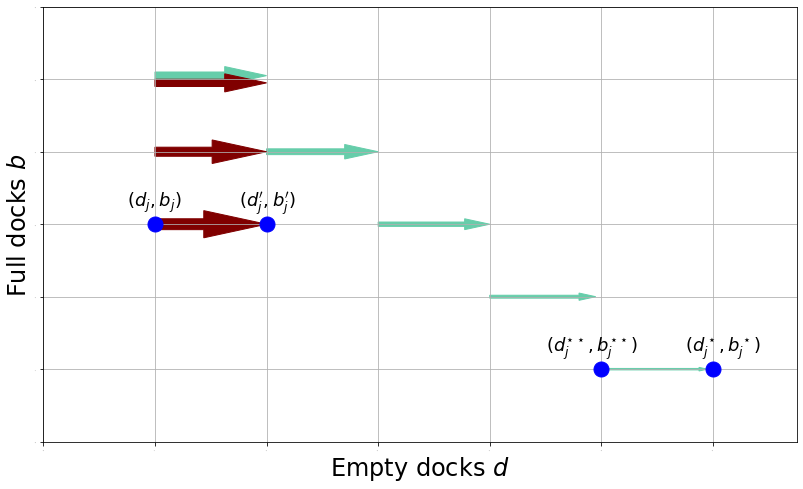}
    \caption{Visual illustration of the inequalities argued for station~$j$ in the proof of Lemma \ref{lemma: neighborhoods}, Case~1.).}
    \label{fig:lemma_3}
\end{figure}



%\vspace{-.25in}

\noindent First, apply Inequality~(3) $t$ times to the RHS to get an upper bound of $$c_j(d_j^\star-1-t,b_j^\star+t)-c_j(d_j^\star-t,b_j^\star+t).$$ Setting $t=d_j^\star-d_j-1\geq 0$, we find that the RHS is bounded above by 
\vspace{-.15in}
\[c_j(d_j,b_j^\star+d_j^\star-d_j-1)-c_j(d_j+1,b_j^\star+d_j^\star-d_j-1).\]
\vspace{-.45in}

\noindent Then, apply Inequality~(6) repeatedly to the LHS shows that $\forall s\geq 0$, the LHS is bounded below by~$c_j(d_j,b_j+s)-c_j(d_j+1,b_j+s)$. Hence, by setting $s=b_j^\star+d_j^\star-d_j-b_j-1$, which is non-negative since $b_j+d_j<b_j^\star+d_j^\star$, we bound the LHS from below by
%\vspace{-.2in}
\[
c_j(d_j,b_j+b_j^\star+d_j^\star-d_j-b_j-1)-c_j(d_j+1,b_j+b_j^\star+d_j^\star-d_j-b_j-1).
\] 
%\vspace{-.5in}

\noindent This equals the upper bound on the RHS and thus proves the desired inequality.
Similarly, to show 
\begin{eqnarray}\label{eqn:above}
c_k (d_k-1,b_k)-c_k(d_k,b_k) \leq c_k(d_k^\star,b_k^\star)-c_k(d_k^\star+1,b_k^\star),
\end{eqnarray}
%\vspace{-.5in}

\noindent we apply Inequality~(3) $d_k-d_k^\star-1$ times to bound the LHS in (\ref{eqn:above}) from above by
$$c_k(d_k^\star,b_k+d_k-d_k^\star-1)-c_k(d_k^\star+1,b_k+d_k-d_k^\star-1).$$
Thereafter, we apply Inequality~(6) $(b_k+d_k)-(d_k^\star+b_k^\star) -1\geq 0$ times to obtain the desired bound.

In Case 3.b), we define $(\vec{d}^{\star\star},\vec{b}^{\star\star})=E_{jk\ell}(\vec{d}^{\star},\vec{b}^{\star})$ and $(\vec{d}',\vec{b}')=O_{kj\ell}(\vec{d},\vec{b})$. Similarly to the first case, we need to show that $c(\vec{d},\vec{b})-c(\vec{d'},\vec{b'})\geq c(\vec{d}^{\star\star},\vec{b}^{\star\star})-c(\vec{d}^{\star},\vec{b}^{\star})$. Since all terms not involving $j,k,$ and~$\ell$ cancel out and the terms involving $j$ and $k$ can be bounded the same way as before, deriving
%\vspace{-.5in}
\begin{eqnarray*}
c_\ell (d_\ell,b_\ell)-c_\ell(d_\ell-1,b_\ell+1) \geq c_\ell(d_\ell^\star+1,b_\ell^\star-1)-c_\ell(d_\ell^\star,b_\ell^\star)
\end{eqnarray*}
%\vspace{-.15in}
\noindent suffices. 
We obtain this (see Figure \ref{fig:lemma_3_ell}) by bounding with $s=b_\ell^\star-b_\ell-1\geq 0$
$$c_\ell (d_\ell,b_\ell)-c_\ell(d_\ell-1,b_\ell+1) \geq 
c_\ell (d_\ell-s,b_\ell+s)-c_\ell(d_\ell-1-s,b_\ell+1+s),$$
which follows from Fact 1 (increasing first derivative), and then bounding the resulting term as
$$c_\ell (d_\ell-b_\ell^\star+b_\ell+1,b_\ell^\star-1)
-c_\ell(d_\ell-b_\ell^\star+b_\ell,b_\ell^\star)\geq c_\ell(d_\ell^\star+1,b_\ell^\star-1)-c_\ell(d_\ell^\star,b_\ell^\star),$$
which follows from rewriting Inequality (3) as $f(d+1,b-1)-f(d,b)\geq f(d,b-1)-f(d-1,b) $ and applying it $(b_\ell+d_\ell)-(b_\ell^\star+d_\ell^\star)\geq0$ times.


This concludes the proof of Lemma \ref{lemma: neighborhoods}. \hfill\halmos

\begin{figure}[ht]
    \centering
    \includegraphics[width=.35\textwidth]{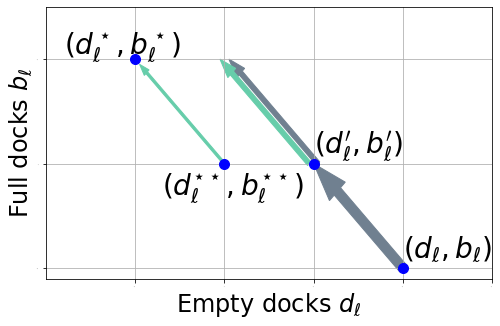}
    \caption{Visual illustration of the sequence of  inequalities argued for station~$\ell$ in the proof of Lemma \ref{lemma: neighborhoods}, Case~3.b).}
    \label{fig:lemma_3_ell}
\end{figure}
%We obtain this  by repeatedly applying inequalities (3) and (4) to the LHS. 

\subsubsection{Proof of Lemma \ref{lemma: exchange}}

The proof of Lemma \ref{lemma: exchange} is almost entirely contained in the constructions of the proof of Lemma~\ref{lemma: neighborhoods} above. The key difference lies in the fact that the argument in the first paragraph of the previous proof assumes that we are indifferent to the specific allocation~$(\vec{d}^{\star},\vec{b}^{\star})$, i.e., we pick any allocation with objective better than $(\vec{d},\vec{b})$, and may thus move along a path towards~$(\vec{d},\vec{b})$, by relabeling allocations as~$(\vec{d}^{\star},\vec{b}^{\star})$,  until we are at the closest allocation with a strictly better objective. This is not permitted in Lemma \ref{lemma: exchange}, and thus we cannot assume that an allocation~$(\vec{d}^{\star\star},\vec{b}^{\star\star})\in N(\vec{d}^{\star},\vec{b}^{\star})$ as described in the first paragraph of the previous proof does not exist. However, the cases in the lemma  defining in each case the same allocations~$(\vec{d}',\vec{b}')$ and~$(\vec{d}^{\star\star},\vec{b}^{\star\star})$ as in Lemma~\ref{lemma: neighborhoods} we find that the second and third condition in the lemma statement are nonetheless fulfilled.  Indeed, the only time we used the specific definition of $(\vec{d}^{\star},\vec{b}^{\star})$ was when arguing that $c(\vec{d}^{\star\star},\vec{b}^{\star\star})<(\vec{d}^{\star},\vec{b}^{\star})$; the proofs of the intermediate inequality $c(\vec{d},\vec{b})-c(\vec{d}',\vec{b}')\geq c(\vec{d}^{\star\star},\vec{b}^{\star\star})-(\vec{d}^{\star},\vec{b}^{\star})$ followed from Definition~\ref{def: multimod} and Lemma~\ref{lemma: multimod} only. 
This guarantees the first condition and concludes the proof of Lemma~\ref{lemma: exchange}.\hfill\halmos
%The constructions in the proof of Lemma \ref{lemma: neighborhoods} fulfill the requirements of Lemma \ref{lemma: exchange}; the only required change is due to the assumption that, without loss of generality, there is no solution $(\vec{d}^{\star\star},\vec{b}^{\star\star})$ that has a better objective than $(\vec{d},\vec{b})$ and is one dock-move closer to $(\vec{d},\vec{b})$ than $(\vec{d}^\star,\vec{b}^\star)$. However, that assumption is only ever used to derive the final inequality in

% $$
% c(\vec{d},\vec{b})-c(\vec{d'},\vec{b'})\geq c(\vec{d}^{\star\star},\vec{b}^{\star\star})-c(\vec{d}^{\star},\vec{b}^{\star})>0.
% $$
